# Supplementary material for: Conditional Noise-Contrastive Estimation of Unnormalised Models
Source: arXiv:1806.03664 source file (2018-06-10)
Supplement: Supplementary file 1 [file supp_images1.pdf]

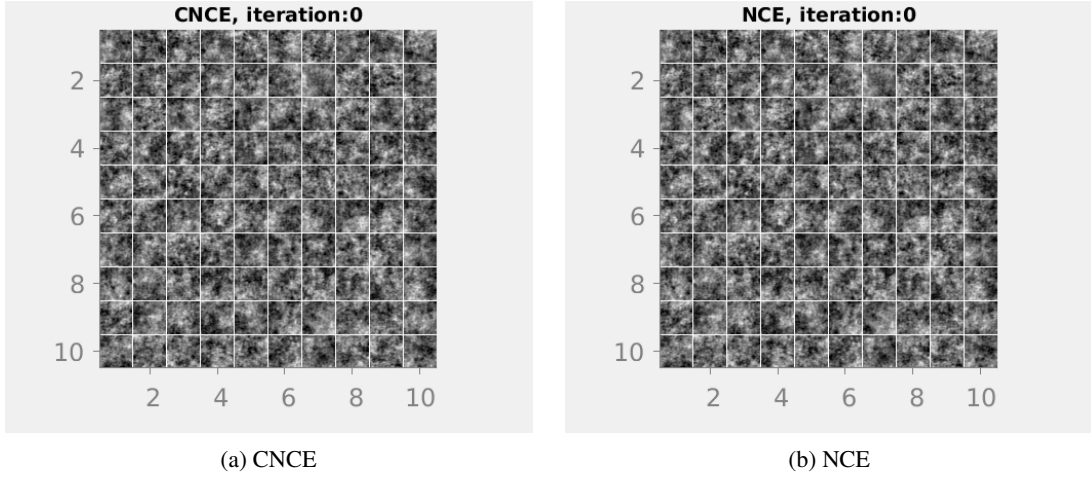

Figure 2: The common initialisation for the 100 1<sup>st</sup> later features used for the qualitative comparison between CNCE and NCE.

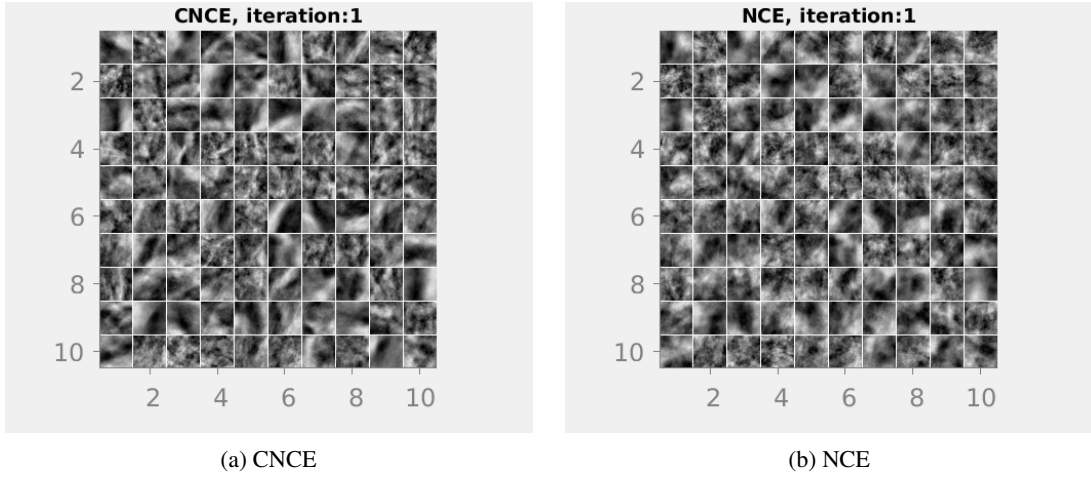

Figure 3: A sample of the 1<sup>st</sup> layer features after 1 meta-iteration.

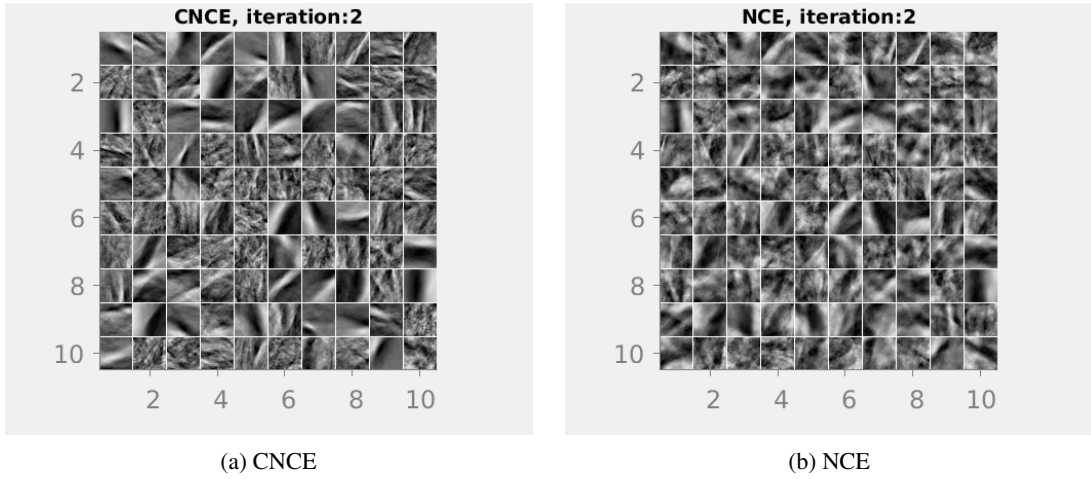

Figure 4: A sample of the 1<sup>st</sup> layer features after 2 meta-iterations.

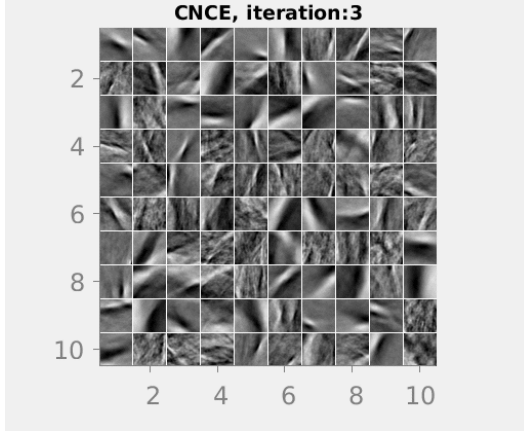

(a) CNCE

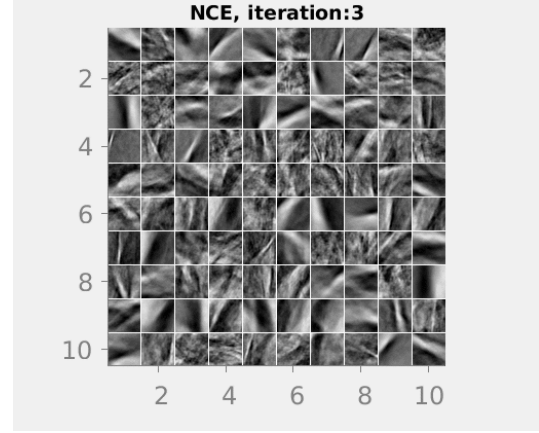

(b) NCE

Figure 5: A sample of the 1<sup>st</sup> layer features after 3 meta-iterations.

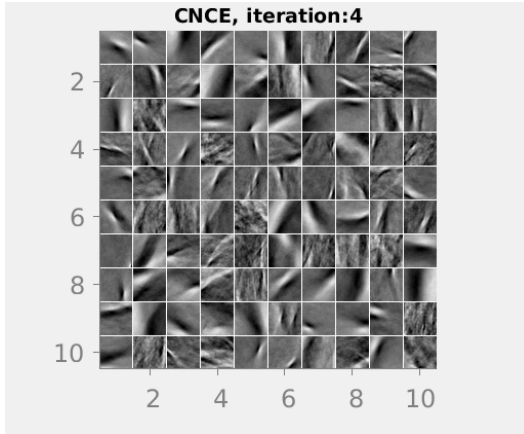

(a) CNCE

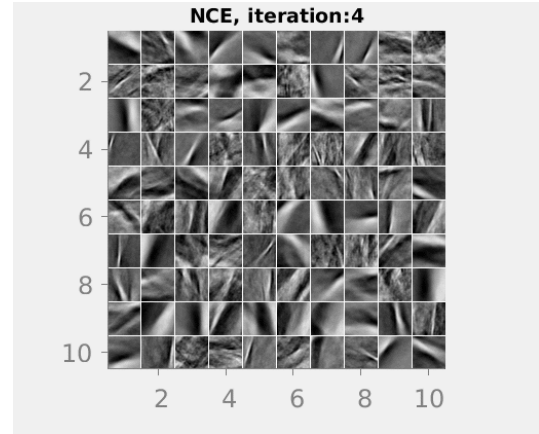

(b) NCE

Figure 6: A sample of the 1<sup>st</sup> layer features after 4 meta-iterations.

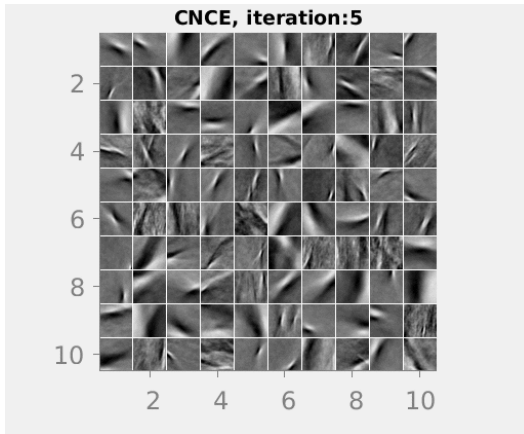

(a) CNCE

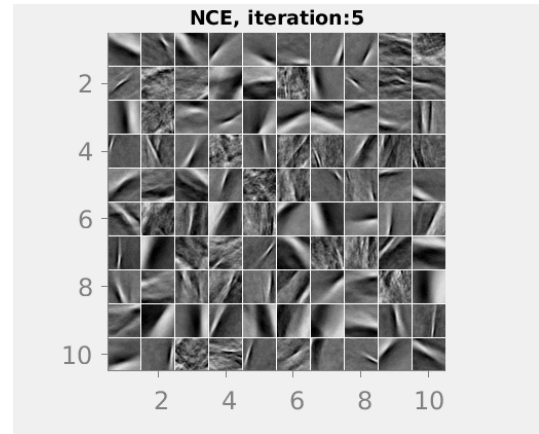

(b) NCE

Figure 7: A sample of the 1<sup>st</sup> layer features after 5 meta-iterations.

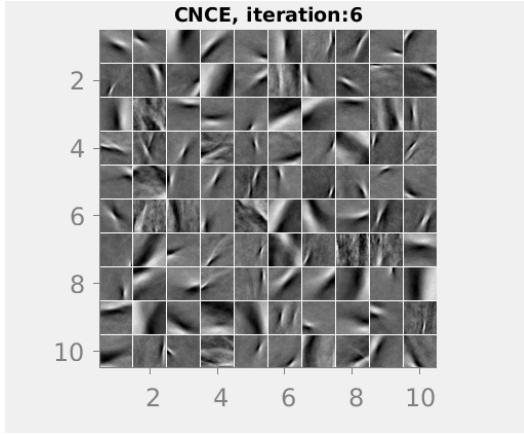

(a) CNCE

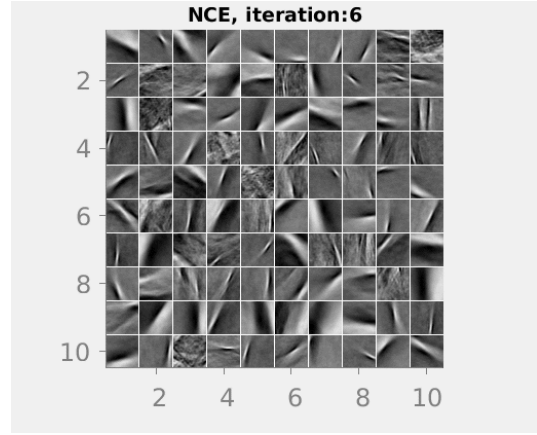

(b) NCE

Figure 8: A sample of the 1<sup>st</sup> layer features after 6 meta-iterations.

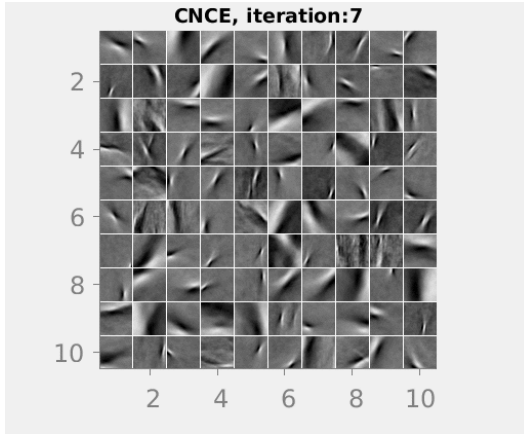

(a) CNCE

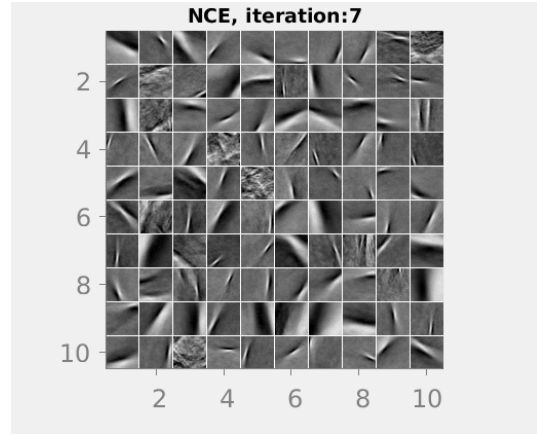

(b) NCE

Figure 9: A sample of the 1<sup>st</sup> layer features after 7 meta-iterations.

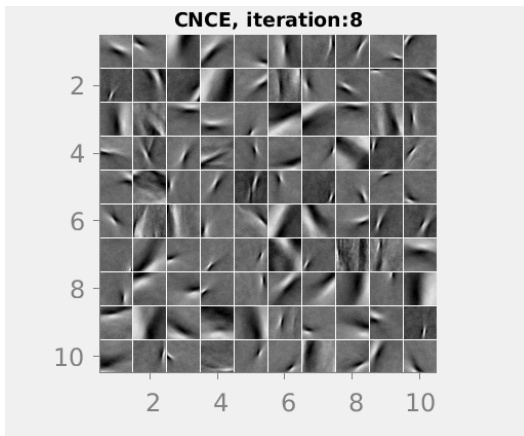

(a) CNCE

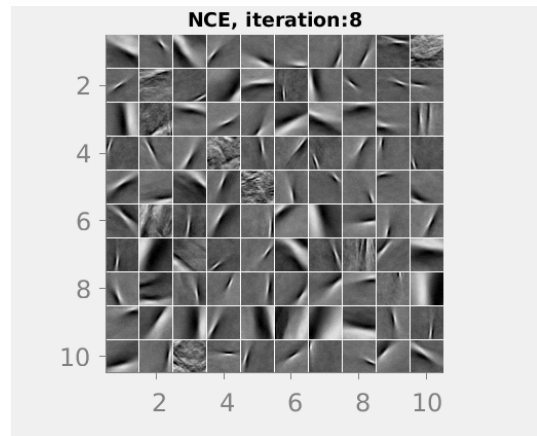

(b) NCE

Figure 10: A sample of the 1<sup>st</sup> layer features after 8 meta-iterations.

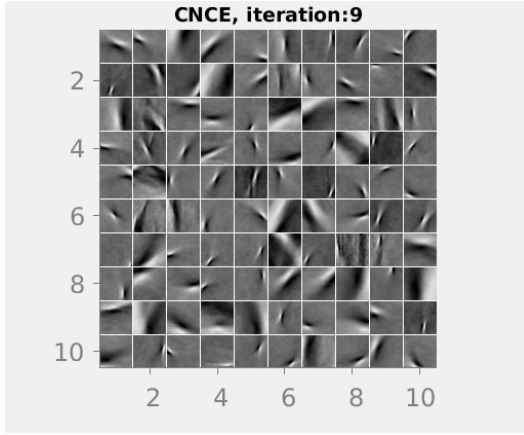

(a) CNCE

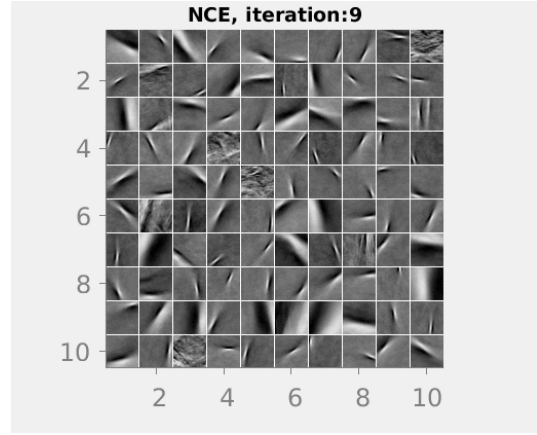

(b) NCE

Figure 11: A sample of the 1<sup>st</sup> layer features after 9 meta-iterations.

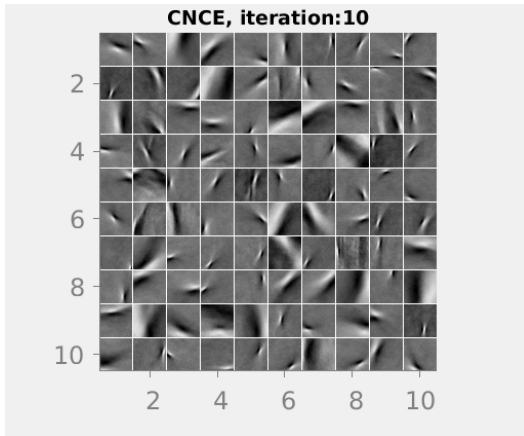

(a) CNCE

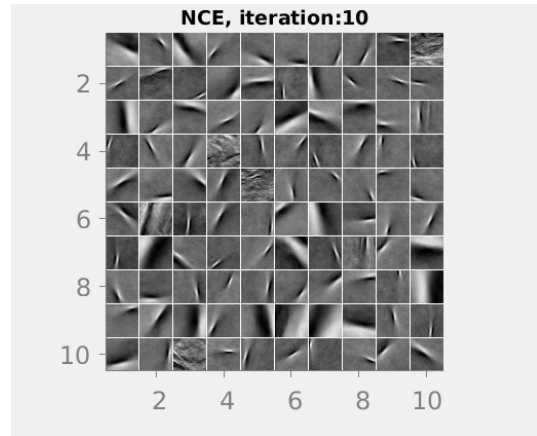

(b) NCE

Figure 12: A sample of the 1<sup>st</sup> layer features after 10 meta-iterations.

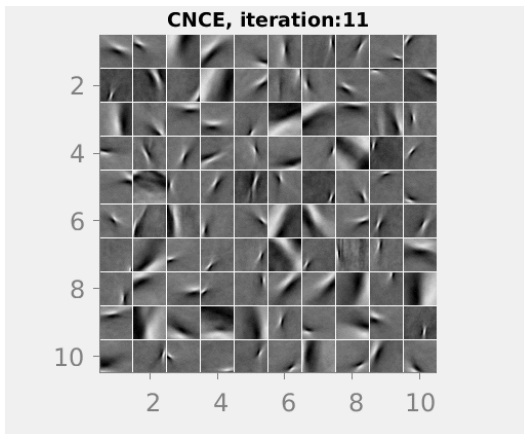

(a) CNCE

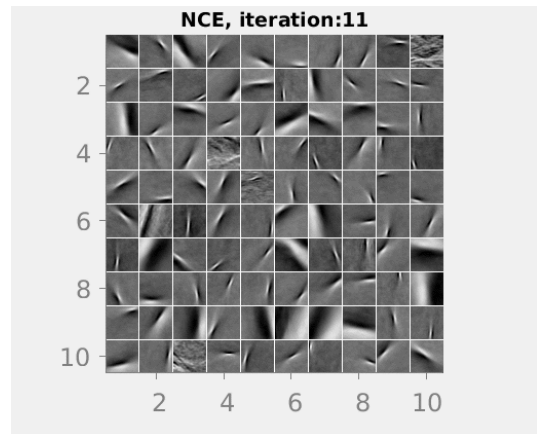

(b) NCE

Figure 13: A sample of the 1<sup>st</sup> layer features after 11 meta-iterations.

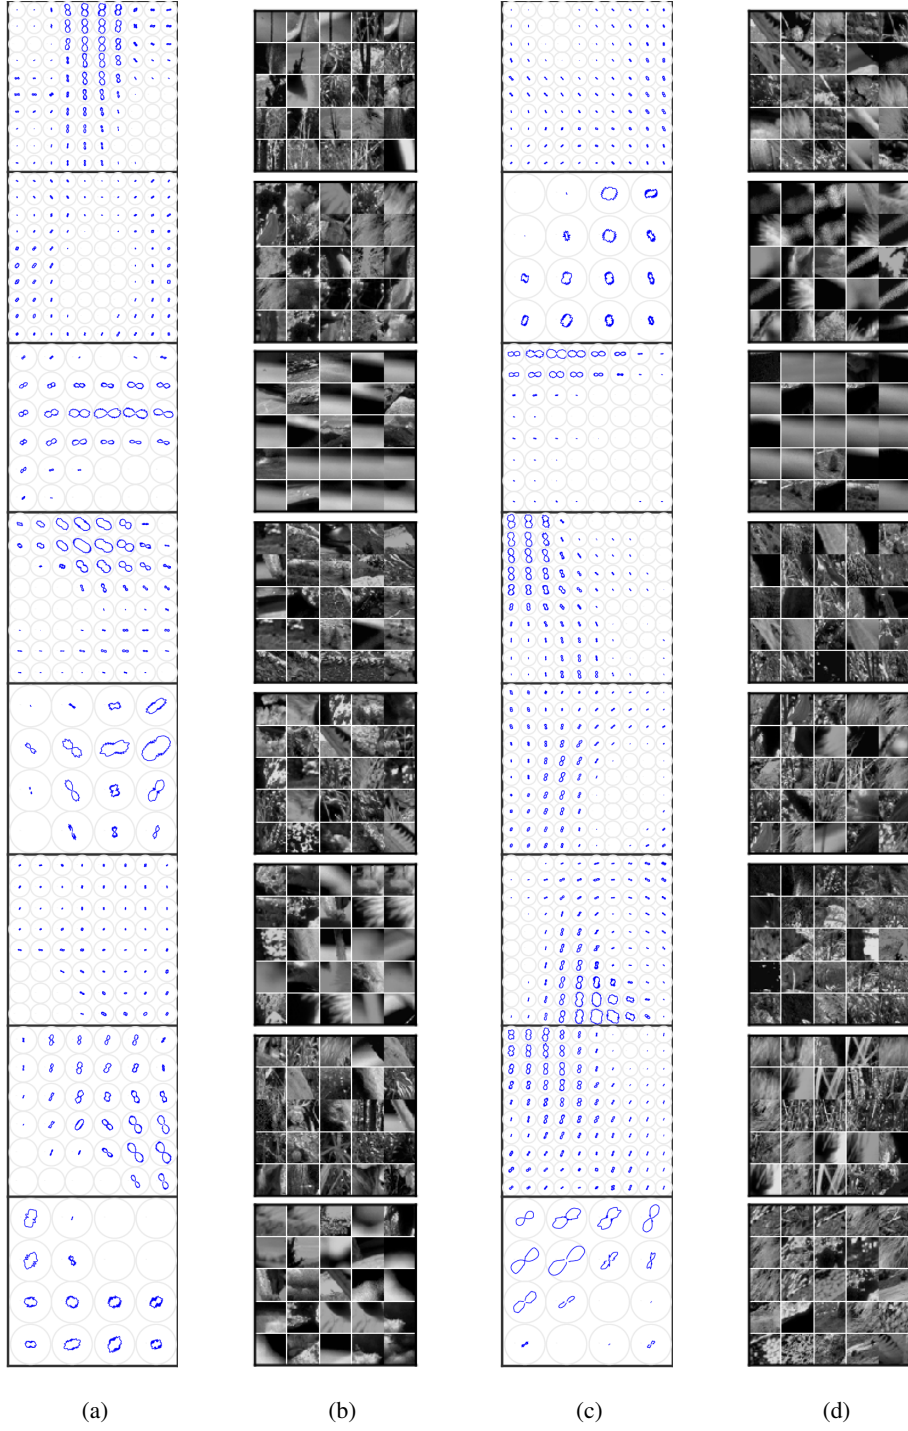

Figure 14: Each row pair of one receptive field and one icon represent a 3<sup>rd</sup> layer unit. (a) and (b) show units 1 to 8, and (c) and (d) 9 to 16.

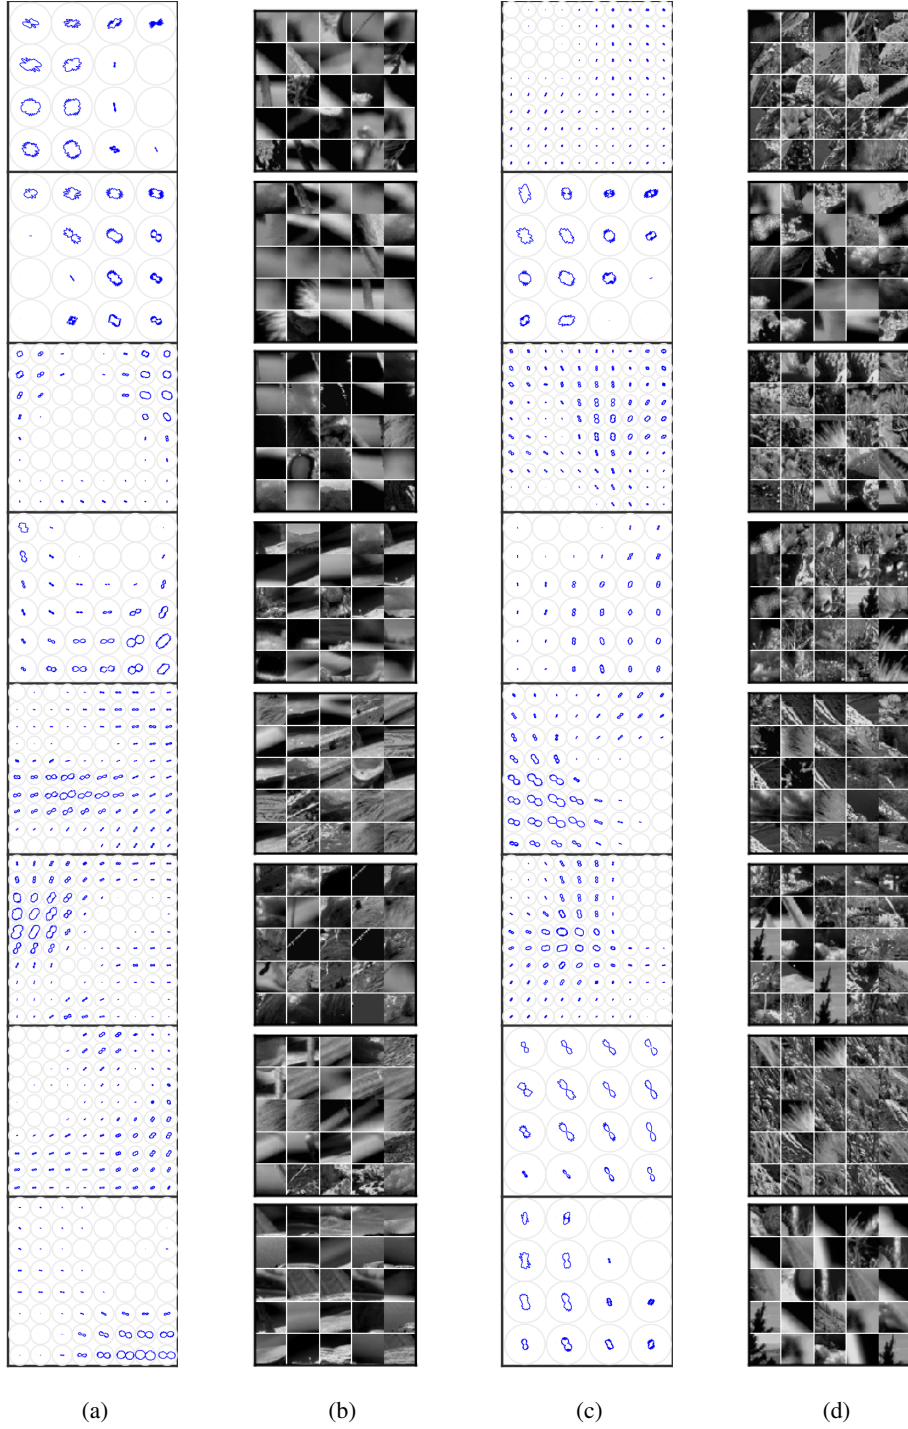

Figure 15: Each row pair of one receptive field and one icon represent a 3<sup>rd</sup> layer unit. (a) and (b) show units 17 to 24, and (c) and (d) 25 to 32.



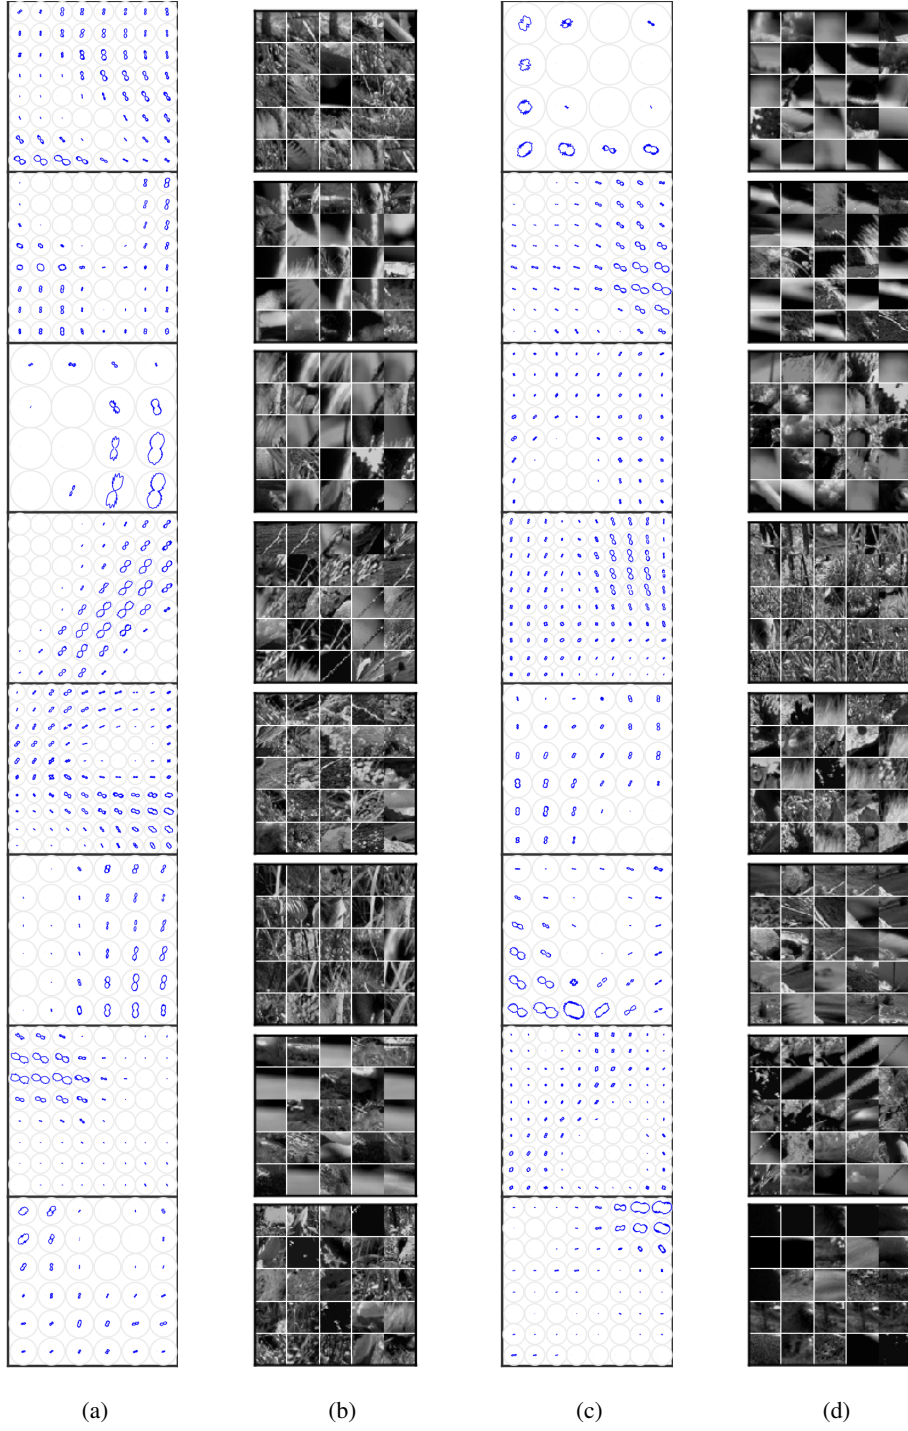

Figure 16: Each row pair of one receptive field and one icon represent a 3<sup>rd</sup> layer unit. (a) and (b) show units 33 to 40, and (c) and (d) 41 to 48.

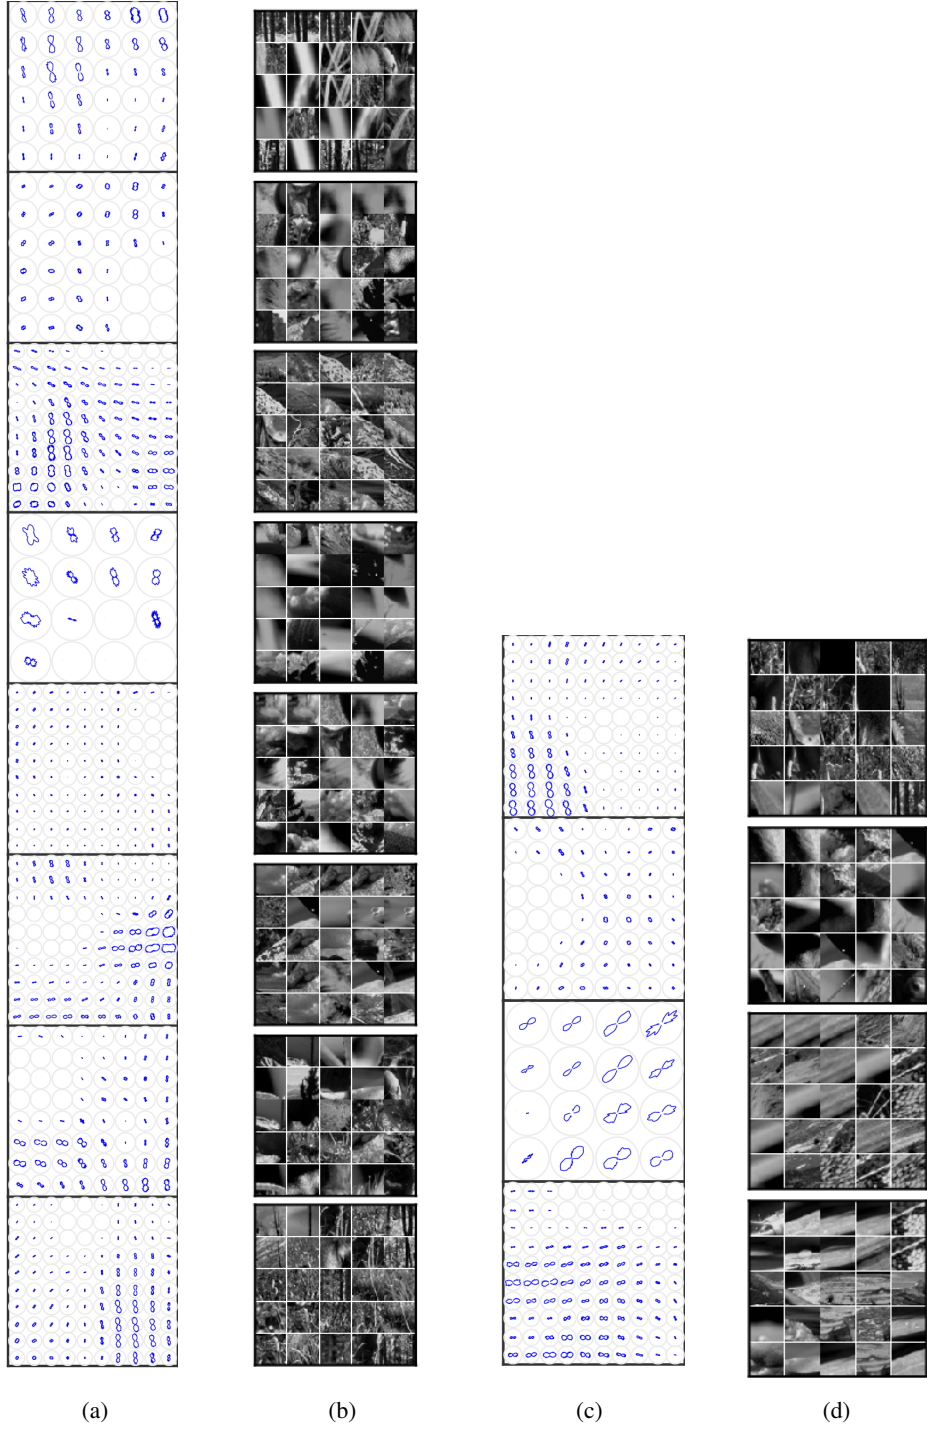

Figure 17: Each row pair of one receptive field and one icon represent a 3<sup>rd</sup> layer unit. (a) and (b) show units 49 to 56, and (c) and (d) 57 to 60.
